# Supplementary material for: Simulation platform for pattern recognition based on reservoir computing with memristor networks
Source: arXiv:2112.00248 source file (2022-06-19)
Supplement: Supplementary file 1 [file supplementary.pdf]

Supplementary Information for

# Simulation platform for pattern recognition based on reservoir computing with memristor networks

Gouhei Tanaka[1,2,3,*] and Ryosho Nakane[2]

[1] International Research Center for Neurointelligence, The University of Tokyo, Tokyo 113-0033, Japan

[2] Department of Electrical Engineering and Information Systems, Graduate School of Engineering, The University of Tokyo, Tokyo 113-8656, Japan

[3] Department of Mathematical Informatics, Graduate School of Information Technology and Science, The University of Tokyo, Tokyo 113-8656, Japan

*Correspondence to: gtanaka@g.ecc.u-tokyo.ac.jp

**This file includes:**

Supplementary Figures 1-7

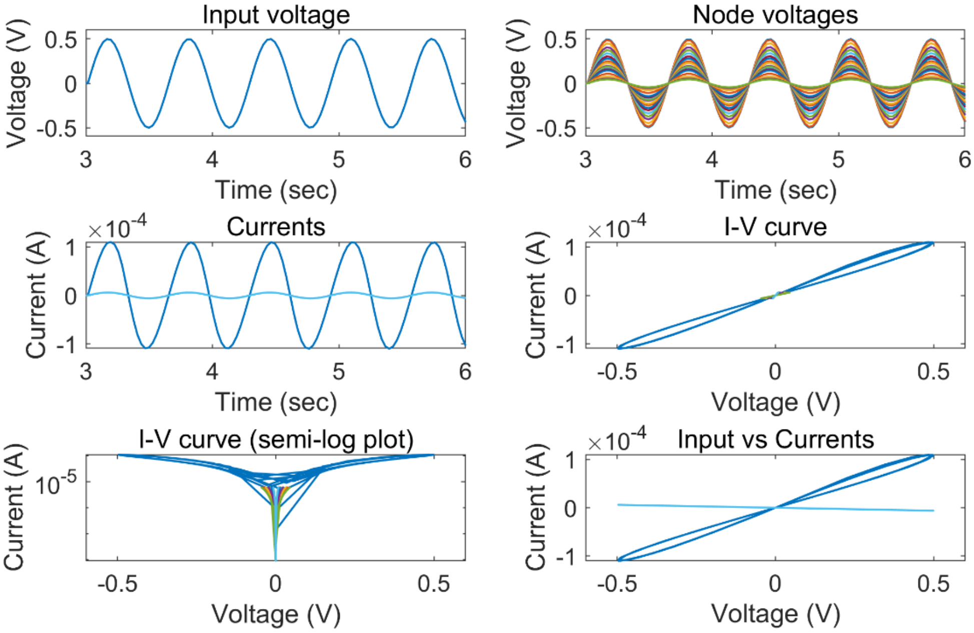


**Supplementary Figure 1: Dynamical behavior of memristor-network-based reservoir driven by a sinusoidal input.** The same as Figure 1, but for a network of the Ring-UP type.

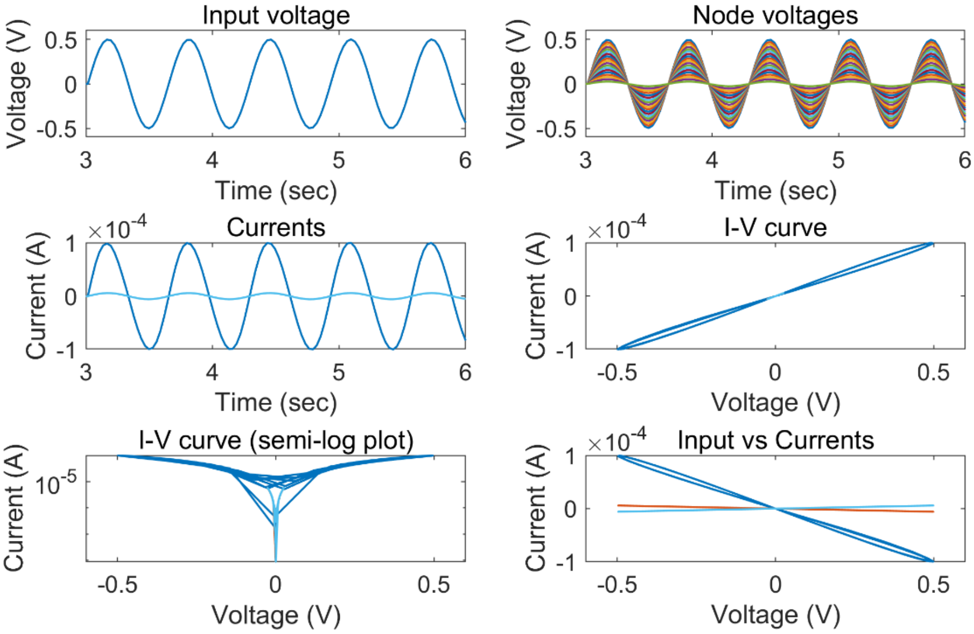


**Supplementary Figure 2: Dynamical behavior of memristor-network-based reservoir driven by a sinusoidal input.** The same as Figure 1, but for a network of the Ring-RP type.

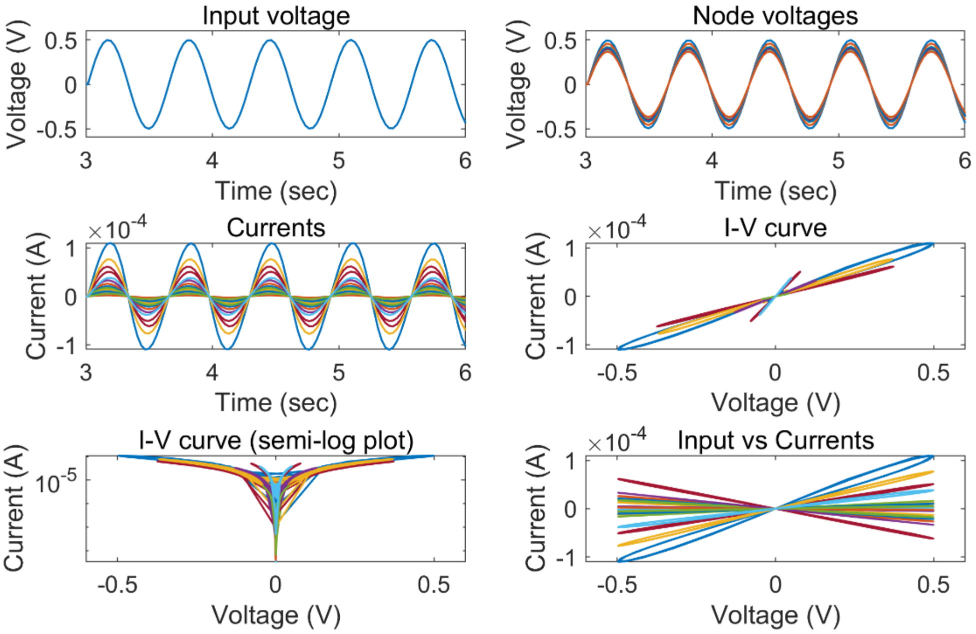


**Supplementary Figure 3: Dynamical behavior of memristor-network-based reservoir driven by a sinusoidal input.** The same as Figure 1, but for a network of the Rand-RP type.

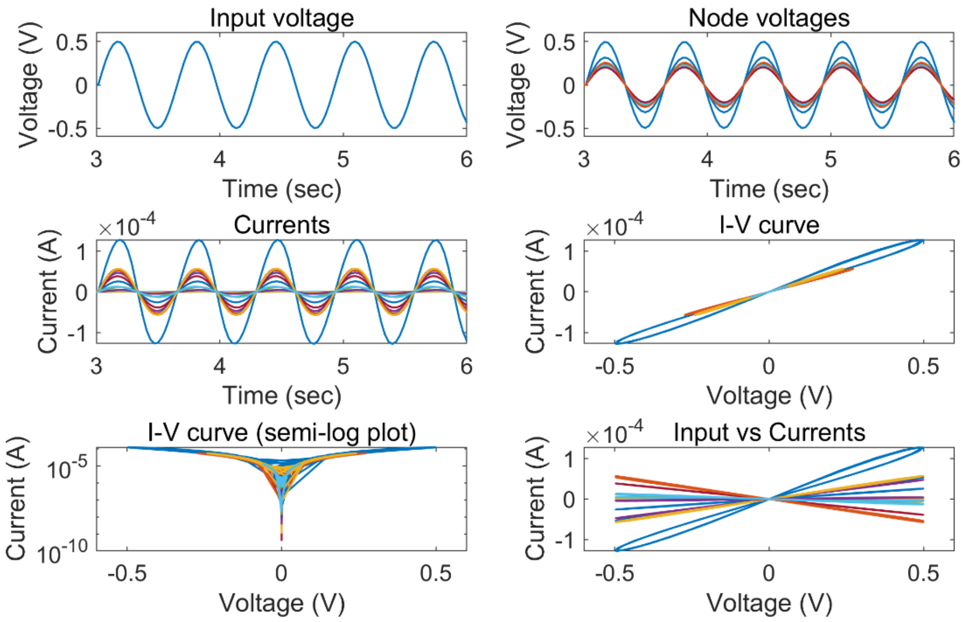


**Supplementary Figure 4: Dynamical behavior of memristor-network-based reservoir driven by a sinusoidal input.** The same as Figure 1, but for the variability parameter set at $\sigma = 0$.

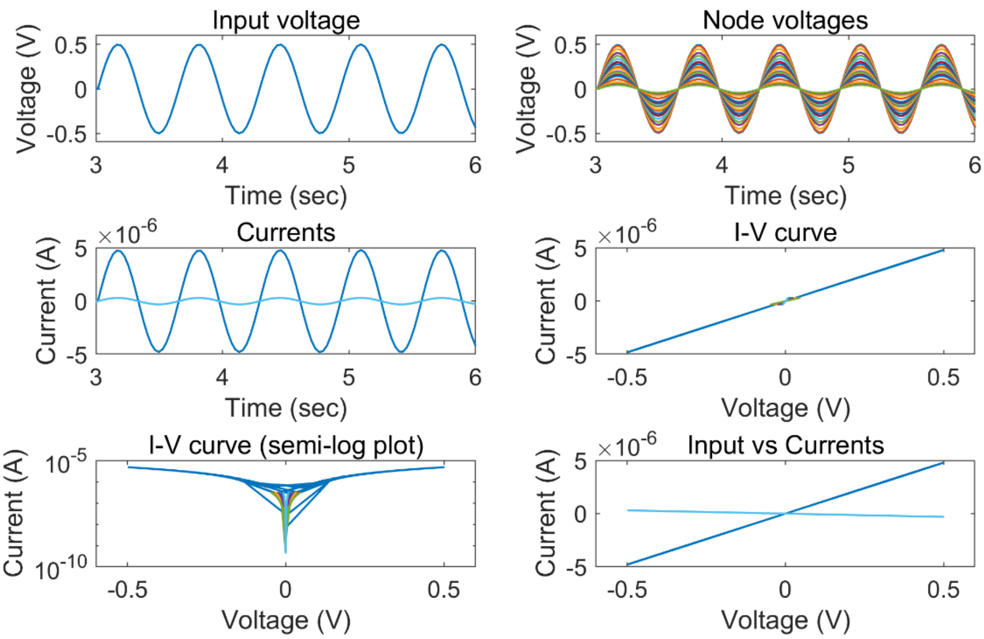


**Supplementary Figure 5: Dynamical behavior of memristor-network-based reservoir driven by a sinusoidal input.** The same as Figure 1, but for the nonlinearity parameter set at $\bar{r} = 10^3$.

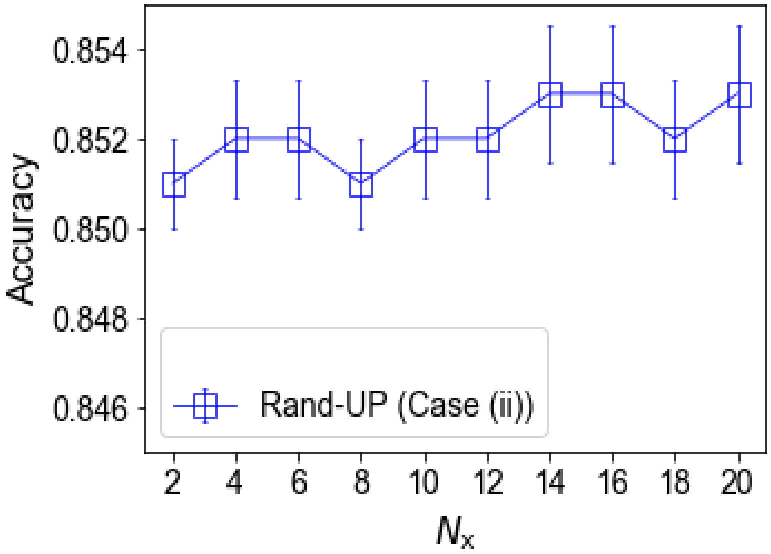


**Supplementary Figure 6: Effect of the number of signals used for the readout in the ECG classification task.** The enlargement of Figure 5c, showing that the performance is slightly improved by increasing $N_\mathrm{x}$ (only for Rand-UP (Case (i)).

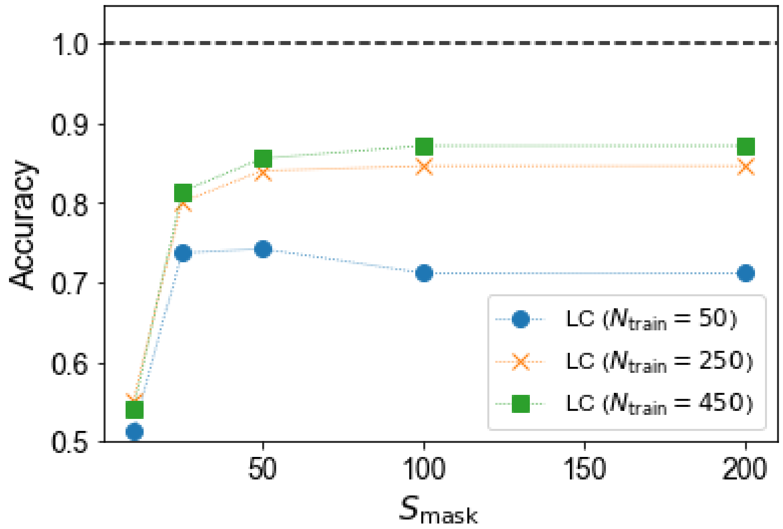


**Supplementary Figure 7: The effect of mask size on the performance of the linear classifier.** The accuracy peaks out at around $S_{\text{mask}} = 100$.
